# Supplementary material for: Unsupervised Imputation of Non-ignorably Missing Data Using Importance-Weighted Autoencoders
Source: arXiv:2101.07357 source file (2022-06-17)
Supplement: Supplementary file 1 [file P2_Appendix-concordance.tex]

\Sconcordance{concordance:P2_Appendix.tex:P2_Appendix.Rnw:%
1 62 1 1 0 319 1}
